# Supplementary material for: Legal and Political Stance Detection of SCOTUS Language
Source: arXiv:2211.11724 source file (2022-11-21)
Supplement: Supplementary file 1 [file aclpubcheck_additional_info.pdf]

Dear Authors,

This year we will make use of `aclpubcheck`, a Python tool that automatically detects author formatting errors, margin violations as well as many other common formatting errors. If you have an accepted paper and it has a formatting violation, you would ordinarily be personalized getting an email from us. However, to see if we can speed things up this year, we are asking you to self-check your paper for formatting violations using a script we developed.

So, we are asking you to ***run the acl_public script*** which is described below ***before*** uploading the camera-ready.

The package is written in Python and there are four steps to using it:
1: `git clone git@github.com:acl-org/aclpubcheck.git or git clone https@github.com:acl-org/aclpubcheck.git`
2: `cd aclpubcheck`
3: `pip install -e .`
4: `python3 aclpubcheck/formatchecker.py --paper_type PAPER_TYPE PAPER_NAME.pdf`

You should also be able to use it via:
1: `pip3 install git+https://github.com/acl-org/aclpubcheck.git`
2: `python3 -m aclpubcheck.formatchecker --paper_type PAPER_TYPE PAPER_NAME.pdf`

We are going to walk you through how to use the tool by considering three papers published by a publication chair at NAACL 2021.

First, consider Josef Valvoda's paper "What About the Precedent: An Information-Theoretic Analysis of Common Law"

```
>> ryans-MBP:ACLPUB ryancotterell$ python3
aclpubcheck/formatchecker.py --paper_type long precedent.pdf

Checking precedent.pdf
Error (Margin): An image on page 1 bleeds into the margin.

We detected 1 error and 0 warnings in your paper.
```

Thus, we see this paper has a margin violation. The script output a png called "errors-precedent-page-1.png" which you can see below:

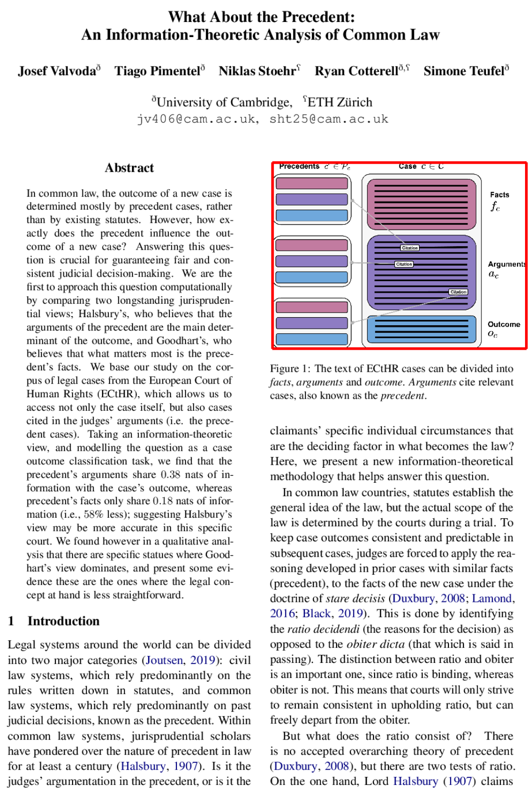

**What About the Precedent:**
**An Information-Theoretic Analysis of Common Law**

**Josef Valvoda**[ð] **Tiago Pimentel**[ð] **Niklas Stoehr**[ς] **Ryan Cotterell**[ð,ς] **Simone Teufel**[ð]

[ð]University of Cambridge, [ς]ETH Zürich
jv406@cam.ac.uk, sht25@cam.ac.uk

**Abstract**

In common law, the outcome of a new case is determined mostly by precedent cases, rather than by existing statutes. However, how exactly does the precedent influence the outcome of a new case? Answering this question is crucial for guaranteeing fair and consistent judicial decision-making. We are the first to approach this question computationally by comparing two longstanding jurisprudential views; Halsbury's, who believes that the arguments of the precedent are the main determinant of the outcome, and Goodhart's, who believes that what matters most is the precedent's facts. We base our study on the corpus of legal cases from the European Court of Human Rights (ECtHR), which allows us to access not only the case itself, but also cases cited in the judges' arguments (i.e. the precedent cases). Taking an information-theoretic view, and modelling the question as a case outcome classification task, we find that the precedent's arguments share 0.38 nats of information with the case's outcome, whereas precedent's facts only share 0.18 nats of information (i.e., 58% less); suggesting Halsbury's view may be more accurate in this specific court. We found however in a qualitative analysis that there are specific statues where Goodhart's view dominates, and present some evidence these are the ones where the legal concept at hand is less straightforward.



Figure 1: The text of ECtHR cases can be divided into *facts*, *arguments* and *outcome*. *Arguments* cite relevant cases, also known as the *precedent*.

**1 Introduction**

Legal systems around the world can be divided into two major categories (Joutsen, 2019): civil law systems, which rely predominantly on the rules written down in statutes, and common law systems, which rely predominantly on past judicial decisions, known as the precedent. Within common law systems, jurisprudential scholars have pondered over the nature of precedent in law for at least a century (Halsbury, 1907). Is it the judges' argumentation in the precedent, or is it the claimants' specific individual circumstances that are the deciding factor in what becomes the law? Here, we present a new information-theoretical methodology that helps answer this question.

In common law countries, statutes establish the general idea of the law, but the actual scope of the law is determined by the courts during a trial. To keep case outcomes consistent and predictable in subsequent cases, judges are forced to apply the reasoning developed in prior cases with similar facts (precedent), to the facts of the new case under the doctrine of *stare decisis* (Duxbury, 2008; Lamond, 2016; Black, 2019). This is done by identifying the *ratio decidendi* (the reasons for the decision) as opposed to the *obiter dicta* (that which is said in passing). The distinction between ratio and obiter is an important one, since ratio is binding, whereas obiter is not. This means that courts will only strive to remain consistent in upholding ratio, but can freely depart from the obiter.

But what does the ratio consist of? There is no accepted overarching theory of precedent (Duxbury, 2008), but there are two tests of ratio. On the one hand, Lord Halsbury (1907) claims

It shows that Josef has to shrink the first-page picture to make the paper compliant with the formatting rules. This is easily remedied with the adjustbox https://www.ctan.org/pkg/adjustbox package or a similar bit of LaTeX.

Next, consider Tiago Pimentel and Irene Nikkarinen's paper: "How (Non-)Optimal is the Lexicon?"

```
>>> python3 aclpubcheck/formatchecker.py --paper_type long
lexicon.pdf

Checking lexicon.pdf
Error (Margin): Text on page 13 bleeds into the margin.
```

This time, the automatically generated png shows me that the authors didn't keep some math equations out of the margin in a proof in the appendix.

| | Train | Validation | Test |
|---|---|---|---|
| English | 242,030 | 66,668 | 66,243 |
| Finnish | 466,745 | 109,232 | 110,378 |
| Hebrew | 311,860 | 104,555 | 104,478 |
| Indonesian | 243,118 | 69,792 | 70,079 |
| Tamil | 479,668 | 116,196 | 115,422 |
| Turkish | 308,419 | 84,300 | 83,871 |
| Yoruba | 47,740 | 12,877 | 12,877 |

Table 3: The number of word types used in training, validation and testing.

## B Model training

As mentioned in the main text, we cannot directly infer the parameters of our model and we use a solution similar to expectation maximization (Wei and Tanner, 1990). We freeze our LSTM generator while learning the PYCRP parameters and then freeze the PYCRP to train the LSTM model.

**Expectation step.** This step uses a Gibbs sampling procedure to estimate the parameters of the PYCRP. For each token in our dataset, we fix all cluster assignments $\mathbf{z}_{-n}$ except for the given token's one $z_n$. We then re-sample this token's cluster based on the marginal probability $p(z_n|\mathbf{z}_{-n}, \boldsymbol{\ell}, \boldsymbol{w}_n)$. We do this for 5 epochs, and use the assignments which result in the best development set cross-entropy. This process can both remove clusters and create new ones by replacing tokens. The set of populated clusters (together with their wordform labels) then allows creating a new wordform dataset of size $K'$, where the distribution of the token frequencies is expected to be less skewed. In practice this can be done by using the resulting set of cluster labels $\{\boldsymbol{\ell}_k\}_{k=1}^{K'}$, i.e. a word will appear in this new dataset as many times as it was assigned as a cluster label.

**Maximization step.** We use the set of populated cluster labels to train the generator LSTM—assuming that this allows learning a more representative model of a language's graphotactics as the irregular common words are less dominant in its training set. In other words, at each epoch, the generator will be trained in a wordform as many times as it has been assigned as a cluster label.

**Hyperparameters and implementation details.** For the PYCRP, we fix hyper-parameters $a = 0.5$ and $b = 10{,}000$, and we use the optimized Gibbs sampling algorithm designed by Blunsom et al. (2009). As our generator, we use a three layers LSTM with an embedding size of 128, a hidden size of 512 and dropout of .33. This LSTM is trained using AdamW (Loshchilov and Hutter, 2019) and we hotstart it by initially training on the set of word types in the training set (the set of unique wordforms in it).

## C Proof of Bounded Entropy for Proposition 2

In this section, we present the proof of Proposition 2. This proposition is repeated here for convenience:

**Proposition 2.** *If a language model $p(\boldsymbol{w})$ is $\varepsilon$-smooth, then its entropy is finite, i.e.* $\mathrm{H}(W) < \infty$.

*Proof.* To prove this, we first break the entropy of a string in two parts. The entropy of the first character, plus the entropy of the following ones given the first.

$$\mathrm{H}(W) = \mathrm{H}(W_1) + \mathrm{H}(W_{>1} \mid W_1) \tag{19}$$

We first bound the entropy of the first character using a uniform distribution upperbound:

$$\begin{aligned}\mathrm{H}(W_1) &= -\sum_{\boldsymbol{w}_1 \in \Sigma} p(\boldsymbol{w}_1) \log p(\boldsymbol{w}_1) \\ &\leq -\log|\Sigma|\end{aligned} \tag{20}$$

We now use the $\varepsilon$-smoothness property to upperbound the entropy of the following characters given the first.

$$\begin{aligned}&\mathrm{H}(W_{>1} \mid W_1) \\ &= \sum_{\boldsymbol{w}_1 \in \Sigma} p(\boldsymbol{w}_1)\mathrm{H}(W_{>1} \mid W_1 = \boldsymbol{w}_1) \\ &= p(\texttt{EoW})\mathrm{H}(W_{>1} \mid W_1 = \texttt{EoW}) \\ &\quad + \sum_{\boldsymbol{w}_1 \in \Sigma, \boldsymbol{w}! = \texttt{EoW}} p(\boldsymbol{w}_1)\mathrm{H}(W_{>1} \mid W_1 = \boldsymbol{w}_1) \\ &= \sum_{\boldsymbol{w}_1 \in \Sigma, \boldsymbol{w}! = \texttt{EoW}} p(\boldsymbol{w}_1)\mathrm{H}(W_{>1} \mid W_1 = \boldsymbol{w}_1) \\ &\leq \sum_{\boldsymbol{w}_1 \in \Sigma, \boldsymbol{w}! = \texttt{EoW}} p(\boldsymbol{w}_1)\mathrm{H}(W_{>1}) \\ &\leq (1-\varepsilon)\,\mathrm{H}(W)\end{aligned} \tag{21}$$

Now that we have both this upperbounds, we can use them to bound the initial equation:

$$\begin{aligned}\mathrm{H}(W) &= \mathrm{H}(W_1) + \mathrm{H}(W_{>1} \mid W_1) \\ &\leq -\log|\Sigma| + (1-\varepsilon)\,\mathrm{H}(W)\end{aligned} \tag{22}$$

Here, it's likely that the equations have to be broken over two lines. But this is okay because ***appendix space is unlimited*** !

Finally, consider Jennifer White's paper "A Non-Linear Structural Probe"

```
python3 aclpubcheck/formatchecker.py --paper_type short
structural.pdf
```

```
Checking structural.pdf
All Clear!
```

So, there were no mistakes!

The script checks for many violations, e.g. page-limit violations, font and font size violations and even a few common typos. The script even makes recommendations about citing non-arXiv versions of papers. These, however, are simply warnings:

```
Warning (Bibliography): It appears you are using arXiv links
more than you should (18/55). Consider using ACL Anthology DOIs
instead.
```

Please send open an issue on github (https://github.com/acl-org/aclpubcheck/issues) if you notice any mistakes or have any suggestions.

**Please check your papers!**
